# Supplementary material for: FetalDiffusion: Pose-Controllable 3D Fetal MRI Synthesis with Conditional Diffusion Model
Source: arXiv:2404.00132 ancillary file (2024-03-29)
Supplement: Supplementary file 1 [file Supplementary.pdf]

# FetalDiffusion: Pose-Controllable 3D Fetal MRI Synthesis with Conditional Diffusion Model: *supplemental document*

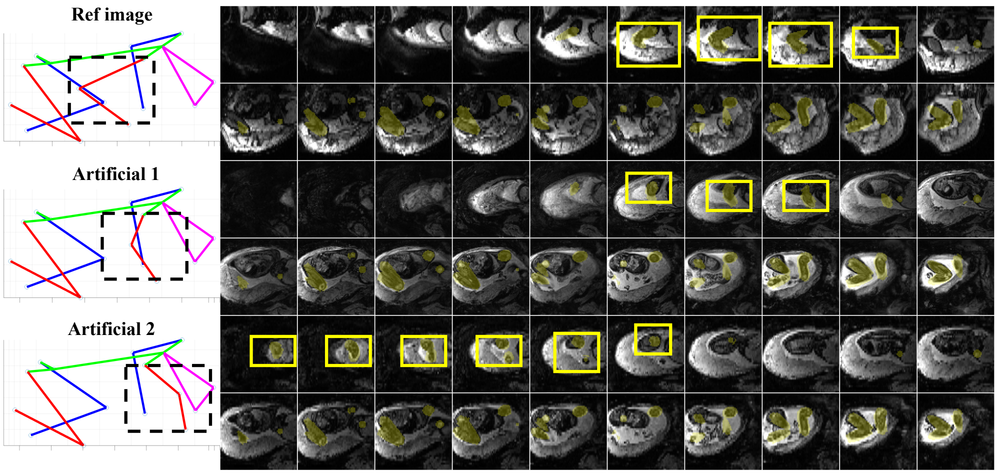


**Fig. S1.** Successful demonstration on unseen poses is illustrated. In the first column, the first row depicts real scanned fetal MRI (reference 1), and we simulate fetal motion by raising the left arm in the second and third rows. For the remaining columns, every two rows correspond to fetal poses on the right. Our proposed method generates high-fidelity images with limbs positioned under the yellow condition mask, emphasizing the arm movements highlighted in the yellow box.

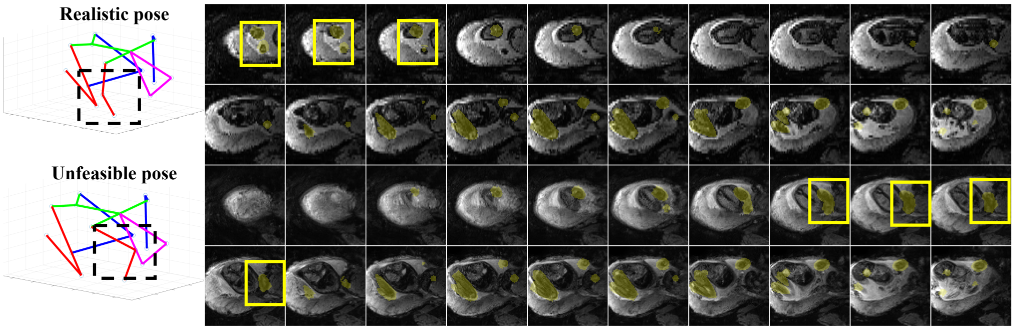


**Fig. S2.** Failure case with an unrealistic pose is presented. Given two similar poses, the first pose features a realistic placement of the left arm, while the second pose exhibits an unrealistic configuration where the elbow is too close to the eyes. The generated images demonstrate that with a realistic pose, our model can generate reasonable and accurate fetal MRI. Conversely, for the unfeasible pose, the fetal brain is contaminated as the arm crosses over it.

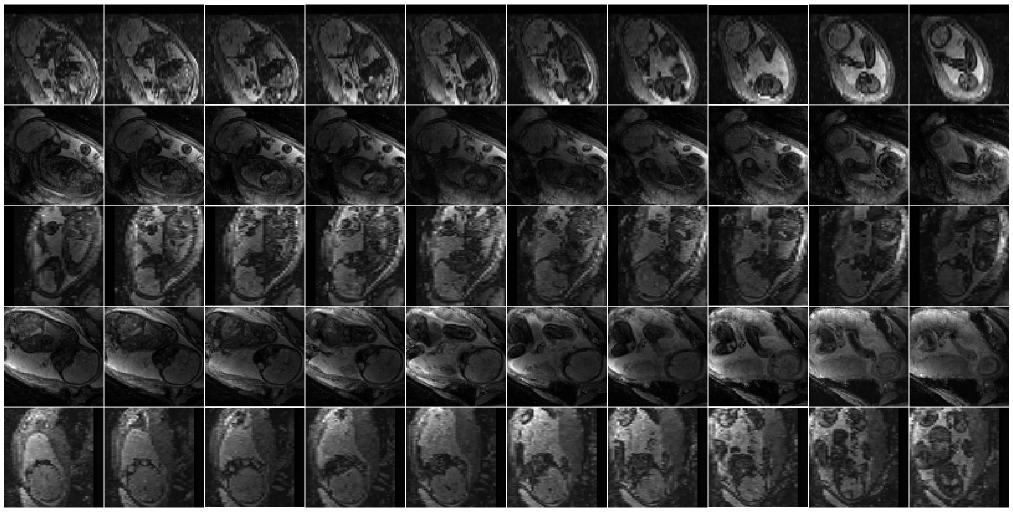

**Fig. S3.** Illustration of generated images as the additional training dataset.
